# Supplementary material for: UnLoc: A Unified Framework for Video Localization Tasks
Source: arXiv:2308.11062 source file (2023-08-21)
Supplement: Supplementary file 1 [file appendix.tex]

% \input{tables/initializations_for_pretraining}

% \input{tables/pretraining_data_scale}
% \input{figures/howto_merge}

% Table ~\ref{tab:initializations_for_pretraining} shows our results on different initializations for pretraining and the effects on zero-shot MR. Interestingly, compared to CLIP + Kinetics + HT-10k, we observe that initializing from CLIP + HT-10k gives btter zero-shot results but worse finetuning results on MR. This suggests that a good zero-shot results cannot be viewed as the single indicator for the final finetuning performance. \arsha{I think this should go into suppl. potentially}
% Table ~\ref{tab:pretraining_data_size} shows our results with different pretraining data scales. We observe the improved performance until 10\% of the HT data. Since the segments duration are shorter than the target datasets (\emph{e.g.} 40.2 seconds in ANet MR and 8.3 second in Charades-STA), we propose to merge segments based on uniform sampling. That is, for each video we randomly sample a number between 1 and K, which will be the number of sentences to merge. Figure \ref{fig:howto_merge} shows the histograms of segment duration under different merging strategies. This allows the merged segment durations to be better matched the target datasets and a significant improvements on zero-shot MR. As shown in row 4-6 and row 10-12 in Table ~\ref{tab:pretraining_data_size}, the improvements are consistent with both HT-10k and HT-100k. 

Table~\ref{tab:hparams} lists all hyperparameters we used for finetuning our models on the four datasets. Note that for COIN dataset we applied sigmoid cross entropy loss and no postprocessing was performance since it is a per-frame prediction task.

\begin{table}[t]
\caption{Finetuning hyperparamters. LR denotes learning rate.}
\centering
\setlength{\tabcolsep}{3pt}
\scriptsize{
\begin{tabular}{lcccc} %
\toprule
 & Charades-STA & ANet-MR & ANet-TAL & COIN \\ \midrule
 \multicolumn{5}{l}{\textit{Training parameters}} \\
Optimizer & \multicolumn{4}{c}{Momentum with rate 0.9}  \\
Gradient clip & \multicolumn{4}{c}{1.0}  \\
Weight decay rate & \multicolumn{4}{c}{1e-4} \\
LR schedule & \multicolumn{4}{c}{Constant with linear warmup} \\
Linear warmup epochs & \multicolumn{4}{c}{2.5} \\
Batch size & \multicolumn{4}{c}{64} \\
Base LR (image/text encoders)	& 0.01 & 0.02 & 0.01 & 0.01 \\
Base LR (video-text fusion + head)	& 0.1 & 0.2 & 0.1 & 0.1 \\
Training epochs	 & 5 & 20 & 20 & 50 \\ \cmidrule{1-5}
\multicolumn{5}{l}{\textit{Data augmentation and regularization}} \\
Random crop probability & \multicolumn{4}{c}{1.0} \\
Random flip probability & \multicolumn{4}{c}{0.5} \\
Scale jitter probability	& \multicolumn{4}{c}{1.0} \\
Maximum scale			  & \multicolumn{4}{c}{1.33} \\
Minimum scale			  & \multicolumn{4}{c}{0.9} \\
Colour jitter probability  & \multicolumn{4}{c}{0.8} \\
Label smoothing~\cite{szegedy_cvpr_2016} & 0.1 & 0.1 & 0.1 & 0.2 \\
RandAugment layers~\cite{cubuk_arxiv_2019} & \multicolumn{4}{c}{3} \\
RandAugment magnitude~\cite{cubuk_arxiv_2019} & \multicolumn{4}{c}{10} \\
Focal loss gamma~\cite{lin2017focal}  & 2.0 & 2.0 & 2.0 & - \\
Focal loss alpha~\cite{lin2017focal}  & 0.25 & 0.25 & 0.25 & - \\ \cmidrule{1-5}
\multicolumn{5}{l}{\textit{Postprocessing}} \\
SoftNMS sigma~\cite{bodla2017soft} & 0.5 & 0.5 & 0.3 & - \\
SoftNMS IoU~\cite{bodla2017soft} & \multicolumn{4}{c}{0.5} \\
\bottomrule
\end{tabular}
}
\label{tab:hparams}
\end{table}
